# Supplementary material for: ARC: Adaptive Robust Joint State and Covariance Estimation
Source: arXiv:2606.20428 source file (2026-06-18)
Supplement: Supplementary file 1 [file appendix.tex]

\section*{Appendix}
